# Supplementary material for: Unconstrained Stochastic CCA: Unifying Multiview and Self-Supervised Learning
Source: arXiv:2310.01012 source file (2024-05-01)
Supplement: Supplementary file 1 [file unfinished_appendices.tex]

\documentclass{article} % For LaTeX2e
\usepackage{iclr2024_conference,times}

% Optional math commands from https://github.com/goodfeli/dlbook_notation.
\input{math_commands.tex}
% Extra maths commands specific to this project
\input{math_commands_lennie.tex}

% Core packages
\usepackage{amsthm}
\usepackage{amsmath}
\usepackage{amssymb}
\usepackage{hyperref}
\usepackage{url}
\usepackage{cleveref}
\usepackage{xr}

% Algorithms
% \RequirePackage{algorithm}
\RequirePackage{algorithmic}
\usepackage[ruled,vlined]{algorithm2e}
\newcommand{\PyComment}[1]{\ttfamily\textcolor{commentcolor}{\# #1}}  % add a "#" before the input text "#1"
\newcommand{\PyCode}[1]{\ttfamily\textcolor{black}{#1}} % \ttfamily is the code font

% packages for graphics and layout
% tables and captions
\usepackage{float}
\usepackage[export]{adjustbox}
\usepackage{booktabs}
\usepackage{caption}
\usepackage{subcaption}
% graphics
\usepackage{graphicx}
\usepackage[inkscapelatex=false]{svg}
\usepackage{wrapfig}
\usepackage{tikz}
\usetikzlibrary{shapes}
\usepackage{xcolor}
\newcommand{\rhexagon}{\mathord{\raisebox{0.6pt}{\tikz{\node[draw,scale=.65,regular polygon, regular polygon sides=6,fill=red](){};}}}}

% theorem environment definitions
% first classic amsthms...
% \newtheorem{proposition}{Proposition}
\newtheorem{corollary}{Corollary}[section]
\newtheorem{definition}{Definition}[section]
\newtheorem{theorem}{Theorem}[section]
\newtheorem{lemma}{Lemma}[section]
\newtheorem{proposition}{Proposition}
\theoremstyle{remark}
\newtheorem*{remark}{Remark}
% then restatable ones
\usepackage{thmtools}
\usepackage{thm-restate}
\declaretheorem[name=Proposition,numberwithin=section]{proprep}


% custom commands that need revising before submission
\newcommand{\lenedit}[1]{\textcolor{teal}{#1}} % fixing problems
%\newcommand{\deleteq}[1]{\textcolor{gray}{#1}} % fixing problems
\newcommand{\citeglassopaper}{\textcolor{red}{cite Lennie Glasso work}}





\begin{document}
\section{Notation Reference}
\subsection{Notation}
We have collected here some notational conventions to help the reader. 
$\norm{\cdot}_2$ denotes the Euclidean norm for vectors.
We shall always have $A,B \in \R^{d\times d}$. Generalised eigenvectors will be denoted by $w$, and CCA directions by $(u,v)$. Related matrices will be denoted by $W,\, (U,V)$ respectively. 
We use $\mathcal{O}(…)$ to denote the asymptotic order of growth of a function, following the standard notation in computer science.
These orders of growth will depend on quantities denoted by the following letters:  $d$ for dimension of GEP, $k$ for dimension of subspace to estimate, $N$ for number of samples, $b$ for minibatch size. 


\newpage
\section{Closer comparison to existing literature}
\subsection{Stochastic Generalised Eigenvalue problems}
Give a more detailed comparison between our method and Chen and Gemp
Expanding out this equation into co-ordinates is helpful for developing intuition for the objective; we have
    \begin{align}\label{eq:EY-charac-intuition}
        \mathcal{L}^\text{EY}(W) \defeq - \underbrace{2 \sum_{k=1}^K w_k^T A w_k}_{\text{Reward}} + \underbrace{\sum_{k=1}^K \left(w_k^T B w_k\right)^2}_{\text{Norm Penalty}} + \underbrace{2 \sum_{1 \leq l < k \leq K} \left(w_l^T B w_k\right)^2}_{\text{Orthogonality Penalty}}
    \end{align}

When presented in this notation, it is clearly related to previous work in \cite{gemp2022generalized}; we discuss these relationships further in ???
In the following sections, we describe a number of algorithms for solving GEPs using proposition \ref{prop:EY-charac}.



\newpage
\section{Analytic forms of GEP formulations of Subspace Learning Application}\label{supp:analyticsubspace}

In this section, we give a short motivation and description for four of the most well-known subspace learning algorithms. 
Subspace learning algorithms are methods that perform dimensionality reduction by finding new variables that capture the most relevant information from the original data. 
In the classical models, these new variables are linear combinations of the original variables, and they form a subspace of the original data space.

For each of our example methods, we can distinguish between a population version of the method (a mathematical object depending on the distribution of some random vectors), and a sample version of the method (where data matrices are used, this can be seen as population object for corresponding empirical distribution).
% In the \textbf{population} case our data are random vectors, whereas in the \textbf{sample} case we have some fixed observations.
It has been argued \cite{arora2012stochastic} that in typical applications of subspace learning methods, we do not have direct access to the distribution over the data with only training `samples' of our data which are treated as random vectors. In this setting we are only able to optimize an estimate the population objective.
On the other hand, the second case leads quickly to algorithm for transforming data (when one has access to some numerical methods) by treating our data as fuxed observations. This final interpretation is how/why these methods are known as and applied as dimensionality reduction methods.

\subsection{Sample Covariance and Population Covariance}
All of the methods can be described through covariance terms: $\mathbb{E}[X^TX]=\Sigma_{XX}$, $\mathbb{E}[Y^TY]=\Sigma_{YY}$, and $\mathbb{E}[X^TY]=\Sigma_{XY}$. We can either consider our training data as samples from the population covariances $\Sigma$ or we can consider the Sample Average Approximation $\frac{1}{b-1}\bar{\mathbf{X}} \bar{\mathbf{Y}}^T=\hat{\Sigma_{XY}}$ where we have a minibatch $b$ of pairs of samples from $X,Y$ into the data matrices $\mathbf{X} \in \R^{p \times b}, \mathbf{Y} \in \R^{q \times b}$ and we let $\bar{\mathbf{X}},\bar{\mathbf{Y}}$ be the centred versions.

\textbf{PCA} is an unsupervised learning algorithm that performs dimensionality reduction by finding new uncorrelated variables that successively maximize variance. These new variables are called principal components and are linear combinations of the original variables. PCA reduces to solving an eigenvalue/eigenvector problem of $\Sigma_{XX}$.

\textbf{LDA} is a supervised learning algorithm that performs dimensionality reduction by finding new variables that maximize the between-class variance while minimizing the within-class variance. These new variables are called linear discriminants and are linear combinations of the original variables. LDA reduces to solving a generalized eigenvalue/eigenvector problem of $\mathbf{S}_B$ and $\mathbf{S}_W$. For LDA, we also need to define the between-class scatter matrix $\mathbf{S}_B$ and the within-class scatter matrix $\mathbf{S}_W$ which in the sample case are:

$$
\hat{\mathbf{S}_B} = \sum_{i=1}^{c} n_i (\mu_i - \mu)(\mu_i - \mu)^T
$$

$$
\hat{\mathbf{S}_W} = \sum_{i=1}^{c} \sum_{x \in X_i} (x - \mu_i)(x - \mu_i)^T
$$

\textbf{PLS} is a multiview learning algorithm that performs dimensionality reduction by finding new variables that maximize the covariance between two sets of variables $X$ and $Y$. These new variables are called partial least squares components and are linear combinations of the original variables. PLS reduces to solving an eigenvalue/eigenvector problem of $A=\begin{pmatrix} 0 & \Sigma_{XY} \\ \Sigma_{YX} & 0 \end{pmatrix}$ and $B=I$. 

\textbf{CCA} is a multiview learning algorithm that performs dimensionality reduction by finding new variables that maximize the correlation between two sets of variables $X$ and $Y$. These new variables are called canonical components and are linear combinations of the original variables. CCA reduces to solving a generalized eigenvalue/eigenvector problem of $A=\begin{pmatrix} 0 & \Sigma_{XY} \\ \Sigma_{YX} & 0\end{pmatrix}$ and $B=\begin{pmatrix} \Sigma_{XX} & 0 \\ 0 & \Sigma_{YY} \end{pmatrix}$.

\textbf{Multi-view CCA} is a straightforward extension of CCA to the case of 3-or more datasets. 
There are various different generalisations of CCA to 3-or-more views in the literature.
But here we describe the most natural GEP-based extension of the two view case. Just write down the relevant $A,B$.
\begin{equation}\label{eq:multi-view-cca-GEV}
	A = \begin{pmatrix} 0 &\Sigma_{XY} & \Sigma_{XZ} \\ \Sigma_{YX} & 0 & \Sigma_{YZ} \\ \Sigma_{ZX} & \Sigma_{ZY} & 0 \end{pmatrix}, \qquad
	B = \begin{pmatrix}\Sigma_{XX} & 0 & 0 \\ 0 & \Sigma_{YY} & 0 \\ 0 & 0 & \Sigma_{ZZ} \end{pmatrix}, \qquad
	w =\begin{pmatrix}	u \\ v \\ w \end{pmatrix}
\end{equation}

Table \ref{tab:subspace} summarizes the definitions of $A$ and $B$ for different subspace learning methods.


%table with PCA, LDA, CCA, PLS and their definitions of A and B e.g. PCA A=X'X B=I.
\begin{table}[ht] 
\centering 
\begin{tabular}{|c|c|c|c|}
\hline 
Method & $A$ & $B$ & $W$\\ 
\hline 
PCA & $\Sigma_{XX}$ & $\mathbf{I}$ & $\begin{pmatrix}W\end{pmatrix}$\\ 
\hline 
LDA & $\mathbf{S}_B$ & $\mathbf{S}_W$  & $\begin{pmatrix}W\end{pmatrix}$\\
\hline 
CCA & $\begin{pmatrix} \Sigma_{XX} & \Sigma_{XY} \\ \Sigma_{YX} & \Sigma_{YY} \end{pmatrix}$ & $\begin{pmatrix} \Sigma_{XX} & 0 \\ 0 & \Sigma_{YY} \end{pmatrix}$ & $\begin{pmatrix} U \\ V \end{pmatrix}$\\
\hline 
PLS & $\begin{pmatrix} 0 & \Sigma_{XY} \\ \Sigma_{YX} & 0 \end{pmatrix}$ & $\mathbf{I}$ & $\begin{pmatrix} U \\ V \end{pmatrix}$ \\ 
\hline 
\end{tabular} 
\caption{Definitions of $A$ and $B$ for different subspace learning methods. $\mathbf{S}_B$ and $\mathbf{S}_W$ are the between and within class scatter matrices. With the exception of PLS, $\textbf{A}$ is always positive semi-definite.} 
\label{tab:subspace} 
\end{table}

\subsection{Why are stochastic GEP updates fast?}\label{sec:fast-stochastic-GEP-updates}

Here we give the details for CCA, our main subspace learning method of interest.
The details for the other subspace learning methods are analogous as simpler, so left for the reader. We can write our unbiased estimates
\begin{align*}
    \hat{A} = \frac{1}{b-1}  \begin{pmatrix}
        0 & \bar{\mathbf{X}} \bar{\mathbf{Y}}^T \\ \bar{\mathbf{Y}} \bar{\mathbf{X}}^T  & 0
    \end{pmatrix}, \quad
    \hat{B} = \frac{1}{b-1} \begin{pmatrix}
        \bar{\mathbf{X}} \bar{\mathbf{X}}^T 0 \\ 0 & \bar{\mathbf{Y}} \bar{\mathbf{Y}}^T
    \end{pmatrix}
\end{align*}
Then we have $\mathbb{E}(\hat{A}) = A, \mathbb{E}(\hat{B}) = B$ and moreover the computations are fast.
Indeed writing $W = \begin{pmatrix}
    U \\ V
\end{pmatrix}$
we get
\begin{align*}
    \hat{A} W = \frac{1}{b-1}  \begin{pmatrix}
        0 & \bar{\mathbf{X}} \bar{\mathbf{Y}}^T \\ \bar{\mathbf{Y}} \bar{\mathbf{X}}^T  & 0
    \end{pmatrix} \begin{pmatrix}
    U \\ V
\end{pmatrix}
= \begin{pmatrix}
    \bar{\mathbf{X}} \bar{\mathbf{Y}}^T V \\ \bar{\mathbf{Y}} \bar{\mathbf{X}}^T U
\end{pmatrix}
\end{align*}
where we indeed have $\bar{\mathbf{Y}}^T V$ costs $\mathcal{O}(b q K)$ to compute and gives a $b \times K$ matrix so subsequent computation of $X (\bar{\mathbf{Y}}^T V)$ costs another $\mathcal{O}(p b K)$.
So indeed overall cost is $\mathcal{O}((p+q) b K) = \mathcal{O}(d b K)$ as claimed in the main text.
The computation for $\hat{B} W$ is analogous.

The examples for our remaining subspace methods are also similar, and left to the reader.

\newpage
\section{Algorithmic Details} \label{supp:algorithm-details}

\subsection{Stochastic Optimization of CCA-SVD}
We next show how CCA-SVD can be efficiently optimized using stochastic methods, which makes them suitable for large-scale and online settings.
Suppose we have an unbiased estimate $\hat{\Sigma}_{XY}$ for $\Sigxy$ and a pair of independent and unbiased estimates $(\hat{\Sigma}_{XY},\hat{\Sigma}_{YY})$ of the matrices $\Sigxx$ and $\Sigyy$ (for example obtained from a minibatch); then one can estimate the objective in proposition \ref{prop:CCA-SVD-charac} by:
\begin{align}
    \mathcal{U}^\text{CCA-SVD}(U,V) 
        \defeq 2 \tr\left(U^T \hat{\Sigma}_{XY} V \right) - \tr\left( U^T \hat{\Sigma}_{XY} U \: V^T \hat{\Sigma}_{YY} V \right)
\end{align}

which we can differentiate to give a gradient estimates:
\begin{align}\label{eq:CCA-SVD-grad-U}
    \hat{\Delta}^{\text{CCA-SVD}}(U)
    \defeq \nabla_U \hat{\mathcal{U}}^\text{CCA-SVD}(U)
    = 2 \hat{\Sigma}_{XY} V - 2\hat{\Sigma}_{XY} U \left(V^T \hat{\Sigma}_{YY} V \right)
\end{align}

\begin{align}\label{eq:CCA-SVD-grad-V}
    \hat{\Delta}^{\text{CCA-SVD}}(V)
    \defeq \nabla_V \hat{\mathcal{U}}^\text{CCA-SVD}(V)
    = 2 \hat{\Sigma}_{YX} U - 2\hat{\Sigma}_{YY} V \left(U^T \hat{\Sigma}_{XX} U \right)
\end{align}

By taking independence $(\hat{\Sigma}_{XY},\hat{\Sigma}_{YY})$ we can obtain unbiased estimates.
These updates immediately leads to Algorithm \ref{alg:Delta-SVD}.
As in Section \ref{sec:fast-stochastic-GEP-updates}, the complexity of each update step is only $\mathcal{O}(b \text{max}(p,q) K)$. 
% It has the added advantage of being slig
% Moreover becauseThe this is potentially as much as half the $\mathcal{O}(n d K)$ complexity of GEY-EY.
%L: I've removed these extra lines because they aren't true anymore if one uses my updates from previous appendix section
% think the advantages of SVD formulation are probably elsewhere really / in the optimisation behaviour

\begin{algorithm}[ht]
\SetAlgoLined
\KwResult{GEP subspace}
 \textbf{Input:} data stream $Z_t$ consisting of B samples from $z_n$. Learning rate $(\eta_t)_t$. Number of time steps $T$. Number of eigenvectors to compute $k$\;
 \textbf{Initialise:} $(\hat{\mathbf {U}})_{i=1}^K$ and $(\hat{\mathbf {V}})_{i=1}^K$ with random uniform entries\;
 \For{$t=1$ \KwTo $T$}{
  Construct an independent unbiased estimate of $\hat{\Sigma}_{XY}$ and independent unbiased estimates of $(\hat{\Sigma}_{XY},\hat{\Sigma}_{YY})$ from $Z_t$\;
  $\hat{\mathbf {U}} \leftarrow \hat{\mathbf {U}}+\eta_{t} \hat{\Delta}^{\text{CCA-SVD}}(U)$ \tcp*{As defined in (\ref{eq:CCA-SVD-grad-U})}
  $\hat{\mathbf {V}} \leftarrow \hat{\mathbf {V}}+\eta_{t} \hat{\Delta}^{\text{CCA-SVD}}(V)$ \tcp*{As defined in (\ref{eq:CCA-SVD-grad-V})}
 }
 \caption{CCA-SVD: A Stochastic Gradient Descent Algorithm for GEP subspace}
 \label{alg:Delta-SVD}
\end{algorithm}


\subsection{DCCA-SVD}\label{sec:deep-cca-svd}

We derive the DCCA-SVD formulation by applying the SVD formulation of CCA to our DCCA definition.

The SVD formulation becomes:
\begin{equation*}
    \hat{\Sigma}_{fg} = \operatorname{Cov}(f(X),g(Y)),\qquad
    \hat{\Sigma}_{ff} = \operatorname{Cov}(f(X),f(X)),\qquad
    \hat{\Sigma}_{gg} =\operatorname{Cov}(g(Y),g(Y))
\end{equation*}

Proposition \ref{prop:CCA-SVD-charac} then allows us to rewrite our objective (\ref{eq:DCCA-Andrew}) as:
\begin{align*}
    \norm{\CCA_k\left(f(X),g(Y)\right)}^2 
    = \sum_{j=1}^k \rho_j^2 
    = \sup_{U,V} \: \tr\left\{2 U^T \hat{\Sigma}_{fg} V  - \left( U^T \hat{\Sigma}_{ff} U \right) \: \left(V^T \hat{\Sigma}_{gg} V \right)\right\}.
\end{align*}
where the supremum is over $U \in \R^{d_x \times K},V \in \R^{d_y \times K}$, consistent with the conventions of the main text.
Therefore DCCA is equivalent to maximising the right hand side with respect to $f,g$ and $W$. To simplify the objective we follow \cite{wang2015stochastic} and reparametrize to consider the `augmented' neural networks $\bar{f} = U^{\top} f, \bar{g} = V^{\top} g$, where $U\in \R^{d_x \times k}, V\in \R^{d_y \times k}$ are such that $W^{\top} = (U^{\top}, V^{\top})$. This gives our final DCCA objective:

\begin{align}\label{eq:DCCA-SVD}
    \mathcal{U}^\text{DCCA-SVD}(\bar{f},\bar{g}) = \tr(2 \, A_{\bar{f}\bar{g}} - B_{\bar{f}\bar{f}} B_{\bar{g}\bar{g}})
\end{align}

where we need to define:
\begin{align*}
    A_{\bar{f}\bar{g}}
    &= U^T A_{fg} V
    = \Cov(\bar{f}(X),\bar{g}(Y)) + \Cov(\bar{g}(Y),\bar{f}(X)) \\
    B_{\bar{f}\bar{f}} 
    &= U^T B_{ff} U 
    = \Cov(\bar{f}(X)) + \Cov(\bar{f}(X)) \\
    B_{\bar{g}\bar{g}} 
    &= V^T B_{gg} V 
    = \Cov(\bar{g}(Y)) + \Cov(\bar{g}(Y))
\end{align*}

By plugging in sample covariances on a minibatch, we can obtain unbiased estimates of $\mathcal{U}^\text{DCCA-SVD}(\bar{f},\bar{g})$. Therefore, we can apply some variant of SGD to optimize equation \ref{eq:DCCA-SVD}.
\end{document}
